# Supplementary material for: Automatic Tensor-level Execution of Abstract Interpreters for Neural Networks
Source: arXiv:2507.20055 source file (2026-10-16)
Supplement: Supplementary file 1 [file appendix.tex]

\begin{figure}
\centering
$
\begin{array}{c}
    \inferrule*[lab = \textsc{Shape-mult-float}]
    {
    \Gamma \vdash \expr_1 \oplus \expr_2 : \types \qquad
    \types \not\in \{\polyexp, \symexp\} \qquad
    \oplus \in \{*, /\} \\\\
    \Gamma, \store_\irshape, \store_\irbroadcast, \fstore \models \expr_1 \goesto \irstatement[1], \irexpression[1], \irm_1 \qquad
    \Gamma, \store_\irshape, \store_\irbroadcast, \fstore \models \expr_2 \goesto \irstatement[2], \irexpression[2], \irm_2 \\\\
    \irexpression[1]', \irexpression[2]', \irm = \matchdims(\irexpression[1], \irexpression[2], \irm_1, \irm_2) 
    }
    {
    \Gamma, \store_\irshape, \store_\irbroadcast, \fstore \models \expr \oplus \expr_2 \goesto \irseq(\irstatement[1], \irstatement[2]), \irmult(\irexpression[1]', \irexpression[2]', \oplus), \irm
    }
\end{array}
$
\caption{Shape analysis for Binary Float}
\label{fig:shapeanalysisbinaryfloat}
\end{figure}

\begin{figure}
\centering
$
\begin{array}{c}
    \inferrule*[lab = \textsc{Shape-binary-symexp}]
    {
    \Gamma \vdash \expr_1 \oplus \expr_2 : \symexp \qquad
    \oplus \in \{+, - \} \\\\
    \Gamma, \store_\irshape, \store_\irbroadcast, \fstore \models \expr_1 \goesto \irstatement[1], \irexpression[1], \irm_1 \qquad
    \Gamma, \store_\irshape, \store_\irbroadcast, \fstore \models \expr_2 \goesto \irstatement[2], \irexpression[2], \irm_2 \\\\
    \irm_1|_\types \in \{\float, \intt \} \implies \irexpression[1]' = \irconstsym(\irexpression[1]) \qquad
    \irm_1|_\types \in \{\typenoise \} \implies \irexpression[1]' = \irnoisesym(\irexpression[1]) \\\\
    \irm_2|_\types \in \{\float, \intt \} \implies \irexpression[2]' = \irconstsym(\irexpression[2]) \qquad
    \irm_2|_\types \in \{\typenoise \} \implies \irexpression[2]' = \irnoisesym(\irexpression[2]) \\\\
    \irexpression[3] = \irextractsymcoeff(\irexpression[1]')\qquad
    \irexpression[4] = \irextractsymcoeff(\irexpression[2]')\\\\
    \irexpression[5] = \irextractsymconst(\irexpression[1]')\qquad
    \irexpression[6] = \irextractsymconst(\irexpression[2]')\\\\
    \irm_3 = \irm_1[\types \mapsto \float][\irshape \mapsto \irm_1(\irshape).append(\syms)][\irbroadcast \mapsto \irm_1(\irbroadcast).append(1)] \\\\ 
    \irm_4 = \irm_2[\types \mapsto \float][\irshape \mapsto \irm_2(\irshape).append(\syms)][\irbroadcast \mapsto \irm_2(\irbroadcast).append(1)] \\\\
    \irm_5 = \irm_1[\types \mapsto \float] \qquad
    \irm_6 = \irm_2[\types \mapsto \float] \\\\
    \irexpression[3]', \irexpression[4]', \irm_7 = \matchdims(\irexpression[3], \irexpression[4], \irm_3, \irm_4) \qquad 
    \irexpression[5]', \irexpression[6]', \irm_8 = \matchdims(\irexpression[5], \irexpression[6], \irm_5, \irm_6) \\\\ 
    \irexpression[7] = \irbinary(\irexpression[3], \irexpression[4], \oplus) \qquad 
    \irexpression[8] = \irbinary(\irexpression[5], \irexpression[6], \oplus) \\\\ 
    \irstatement = \irseq(\irstatement[1], \irstatement[2]) \qquad
    \irexpression = \ircombinesym(\irexpression[7], \irexpression[8]) \qquad 
    \irm = \irm_8 
    }
    {
    \Gamma, \store_\irshape, \store_\irbroadcast, \fstore \models \expr \oplus \expr_2 \goesto \irstatement, \irexpression, \irm
    } 
\end{array}
$
\caption{Shape analysis rules Binary SymExp}
\label{fig:shapeanalysisbinarysymexp}
\end{figure}

\begin{figure}
\centering
$
\begin{array}{c}
    \inferrule*[lab = \textsc{Shape-mult-polyexp-lhs}]
    {
    \Gamma \vdash \expr_1 \oplus \expr_2 : \polyexp \qquad
    \Gamma \vdash \expr_1 : \float \qquad
    \oplus \in \{*, / \} \\\\
    \Gamma, \store_\irshape, \store_\irbroadcast, \fstore \models \expr_1 \goesto \irstatement[1], \irexpression[1], \irm_1 \qquad
    \Gamma, \store_\irshape, \store_\irbroadcast, \fstore \models \expr_2 \goesto \irstatement[2], \irexpression[2], \irm_2 \\\\
    \irm_2|_\types = \polyexp  \implies \irexpression[2]' = \irexpression[2] \qquad
    \irm_2|_\types = \typeneuron \implies \irexpression[2]' = \irneuronpoly(\irexpression[2]) \\\\
    \irexpression[3] = \irextractpolyconst(\irexpression[2]')\qquad
    \irexpression[4] = \irextractpolycoeff(\irexpression[2]')\\\\
    \irm_3 = \irm_2[\types \mapsto \float] \qquad
    \irm_4 = \irm_2[\types \mapsto \float][\irshape \mapsto \irm_2(\irshape).append(\polys)][\irbroadcast \mapsto \irm_2(\irbroadcast).append(1)] \\\\
    \irexpression[5], \irexpression[6], \irm_5 = \matchdims(\irexpression[1], \irexpression[3], \irm_1, \irm_3) \qquad 
    \irexpression[7], \irexpression[8], \irm_7 = \matchdims(\irexpression[1], \irexpression[4], \irm_1, \irm_4) \\\\ 
    \irexpression[9] = \irmult(\irexpression[5], \irexpression[6], \oplus) \qquad 
    \irexpression[10] = \irmult(\irexpression[7], \irexpression[8], \oplus) \\\\ 
    \irstatement = \irseq(\irstatement[1], \irstatement[2]) \qquad
    \irexpression = \ircombinepoly(\irexpression[9], \irexpression[10]) \qquad 
    \irm = \irm_5 
    }
    {
    \Gamma, \store_\irshape, \store_\irbroadcast, \fstore \models \expr \oplus \expr_2 \goesto \irstatement, \irexpression, \irm
    } 
    \\\\
    \inferrule*[lab = \textsc{Shape-mult-polyexp-rhs}]
    {
    \Gamma \vdash \expr_1 \oplus \expr_2 : \polyexp \qquad
    \Gamma \vdash \expr_1 : \float \qquad
    \oplus \in \{*, / \} \\\\
    \Gamma, \store_\irshape, \store_\irbroadcast, \fstore \models \expr_1 \goesto \irstatement[1], \irexpression[1], \irm_1 \qquad
    \Gamma, \store_\irshape, \store_\irbroadcast, \fstore \models \expr_2 \goesto \irstatement[2], \irexpression[2], \irm_2 \\\\
    \irm_1|_\types = \polyexp  \implies \irexpression[1]' = \irexpression[1] \qquad
    \irm_1|_\types = \typeneuron \implies \irexpression[1]' = \irneuronpoly(\irexpression[1]) \\\\
    \irexpression[3] = \irextractpolyconst(\irexpression[1]')\qquad
    \irexpression[4] = \irextractpolycoeff(\irexpression[1]')\\\\
    \irm_3 = \irm_1[\types \mapsto \float] \qquad
    \irm_4 = \irm_1[\types \mapsto \float][\irshape \mapsto \irm_1(\irshape).append(\polys)][\irbroadcast \mapsto \irm_1(\irbroadcast).append(1)] \\\\
    \irexpression[5], \irexpression[6], \irm_5 = \matchdims(\irexpression[3], \irexpression[2], \irm_3, \irm_2) \qquad 
    \irexpression[7], \irexpression[8], \irm_7 = \matchdims(\irexpression[4], \irexpression[2], \irm_4, \irm_2) \\\\ 
    \irexpression[9] = \irmult(\irexpression[5], \irexpression[6], \oplus) \qquad 
    \irexpression[10] = \irmult(\irexpression[7], \irexpression[8], \oplus) \\\\ 
    \irstatement = \irseq(\irstatement[1], \irstatement[2]) \qquad
    \irexpression = \ircombinepoly(\irexpression[9], \irexpression[10]) \qquad 
    \irm = \irm_5 
    }
    {
    \Gamma, \store_\irshape, \store_\irbroadcast, \fstore \models \expr \oplus \expr_2 \goesto \irstatement, \irexpression, \irm
    } 
    \\\\
    \inferrule*[lab = \textsc{Shape-mult-symexp-lhs}]
    {
    \Gamma \vdash \expr_1 \oplus \expr_2 : \symexp \qquad
    \Gamma \vdash \expr_1 : \float \qquad
    \oplus \in \{*, / \} \\\\
    \Gamma, \store_\irshape, \store_\irbroadcast, \fstore \models \expr_1 \goesto \irstatement[1], \irexpression[1], \irm_1 \qquad
    \Gamma, \store_\irshape, \store_\irbroadcast, \fstore \models \expr_2 \goesto \irstatement[2], \irexpression[2], \irm_2 \\\\
    \irm_2|_\types = \symexp  \implies \irexpression[2]' = \irexpression[2] \qquad
    \irm_2|_\types = \typenoise \implies \irexpression[2]' = \irnoisesym(\irexpression[2]) \\\\
    \irexpression[3] = \irextractsymconst(\irexpression[2]')\qquad
    \irexpression[4] = \irextractsymcoeff(\irexpression[2]')\\\\
    \irm_3 = \irm_2[\types \mapsto \float] \qquad
    \irm_4 = \irm_2[\types \mapsto \float][\irshape \mapsto \irm_2(\irshape).append(\syms)][\irbroadcast \mapsto \irm_2(\irbroadcast).append(1)] \\\\
    \irexpression[5], \irexpression[6], \irm_5 = \matchdims(\irexpression[1], \irexpression[3], \irm_1, \irm_3) \qquad 
    \irexpression[7], \irexpression[8], \irm_7 = \matchdims(\irexpression[1], \irexpression[4], \irm_1, \irm_4) \\\\ 
    \irexpression[9] = \irmult(\irexpression[5], \irexpression[6], \oplus) \qquad 
    \irexpression[10] = \irmult(\irexpression[7], \irexpression[8], \oplus) \\\\ 
    \irstatement = \irseq(\irstatement[1], \irstatement[2]) \qquad
    \irexpression = \ircombinesym(\irexpression[9], \irexpression[10]) \qquad 
    \irm = \irm_5 
    }
    {
    \Gamma, \store_\irshape, \store_\irbroadcast, \fstore \models \expr_0 \ ? \ \expr_1 \ : \ \expr_2 \goesto \irstatement, \irexpression, \irm
    } 
    \\\\
    \inferrule*[lab = \textsc{Shape-mult-symexp-rhs}]
    {
    \Gamma \vdash \expr_1 \oplus \expr_2 : \symexp \qquad
    \Gamma \vdash \expr_1 : \float \qquad
    \oplus \in \{*, / \} \\\\
    \Gamma, \store_\irshape, \store_\irbroadcast, \fstore \models \expr_1 \goesto \irstatement[1], \irexpression[1], \irm_1 \qquad
    \Gamma, \store_\irshape, \store_\irbroadcast, \fstore \models \expr_2 \goesto \irstatement[2], \irexpression[2], \irm_2 \\\\
    \irm_1|_\types = \symexp  \implies \irexpression[1]' = \irexpression[1] \qquad
    \irm_1|_\types = \typenoise \implies \irexpression[1]' = \irnoisesym(\irexpression[1]) \\\\
    \irexpression[3] = \irextractsymconst(\irexpression[1]')\qquad
    \irexpression[4] = \irextractsymcoeff(\irexpression[1]')\\\\
    \irm_3 = \irm_1[\types \mapsto \float] \qquad
    \irm_4 = \irm_1[\types \mapsto \float][\irshape \mapsto \irm_1(\irshape).append(\syms)][\irbroadcast \mapsto \irm_1(\irbroadcast).append(1)] \\\\
    \irexpression[5], \irexpression[6], \irm_5 = \matchdims(\irexpression[3], \irexpression[2], \irm_3, \irm_2) \qquad 
    \irexpression[7], \irexpression[8], \irm_7 = \matchdims(\irexpression[4], \irexpression[2], \irm_4, \irm_2) \\\\ 
    \irexpression[9] = \irmult(\irexpression[5], \irexpression[6], \oplus) \qquad 
    \irexpression[10] = \irmult(\irexpression[7], \irexpression[8], \oplus) \\\\ 
    \irstatement = \irseq(\irstatement[1], \irstatement[2]) \qquad
    \irexpression = \ircombinesym(\irexpression[9], \irexpression[10]) \qquad 
    \irm = \irm_5 
    }
    {
    \Gamma, \store_\irshape, \store_\irbroadcast, \fstore \models \expr \oplus \expr_2 \goesto \irstatement, \irexpression, \irm
    } 
\end{array}
$
\caption{Shape analysis rules 2}
\label{fig:shapeanalysis2}
\end{figure}

\begin{figure}
\centering
$
\begin{array}{c}
    \inferrule*[lab = \textsc{Shape-ternary-float}]
    {
    \Gamma \vdash \expr_1 \ ? \ \expr_2 \ : \ \expr_3 : \types \qquad
    \types \not\in \{\polyexp, \symexp\} \\\\
    \Gamma, \store_\irshape, \store_\irbroadcast, \fstore \models \expr_1 \goesto \irstatement[1], \irexpression[1], \irm_1 \qquad
    \Gamma, \store_\irshape, \store_\irbroadcast, \fstore \models \expr_2 \goesto \irstatement[2], \irexpression[2], \irm_2 \qquad
    \Gamma, \store_\irshape, \store_\irbroadcast, \fstore \models \expr_3 \goesto \irstatement[3], \irexpression[3], \irm_3 \\\\
    \irexpression[1]', \irexpression[2]', \irm_1 = \matchdims(\irexpression[1], \irexpression[2], \irm_1, \irm_2) \\\\
    \irexpression[1]'', \irexpression[3]', \irm_2 = \matchdims(\irexpression[1]', \irexpression[3], \irm_1, \irm_3) \\\\
    \irexpression[2]'', \irexpression[3]'', \irm_3 = \matchdims(\irexpression[2]', \irexpression[3]', \irm_1, \irm_2) 
    }
    {
    \Gamma, \store_\irshape, \store_\irbroadcast, \fstore \models \expr_1 \ ? \ \expr_2 \ : \ \expr_3 \goesto \irseq(\irseq(\irstatement[1], \irstatement[2]), \irstatement[3]), \irternary(\irexpression[1]'', \irexpression[2]'', \irexpression[3]''), \irm_3
    } 
    \\\\
    \inferrule*[lab = \textsc{Shape-ternary-polyexp}]
    {
    \Gamma \vdash \expr_0 \ ? \ \expr_1 \ : \ \expr_2 : \polyexp \\\\
    \Gamma, \store_\irshape, \store_\irbroadcast, \fstore \models \expr_0 \goesto \irstatement[0], \irexpression[0], \irm_0 \qquad
    \Gamma, \store_\irshape, \store_\irbroadcast, \fstore \models \expr_1 \goesto \irstatement[1], \irexpression[1], \irm_1 \qquad
    \Gamma, \store_\irshape, \store_\irbroadcast, \fstore \models \expr_2 \goesto \irstatement[2], \irexpression[2], \irm_2 \\\\
    \irm_1|_\types \in \{\float, \intt \} \implies \irexpression[1]' = \irconstpoly(\irexpression[1]) \qquad
    \irm_1|_\types \in \{\typeneuron \} \implies \irexpression[1]' = \irneuronpoly(\irexpression[1]) \\\\
    \irm_2|_\types \in \{\float, \intt \} \implies \irexpression[2]' = \irconstpoly(\irexpression[2]) \qquad
    \irm_2|_\types \in \{\typeneuron \} \implies \irexpression[2]' = \irneuronpoly(\irexpression[2]) \\\\
    \irexpression[3] = \irextractpolycoeff(\irexpression[1]')\qquad
    \irexpression[4] = \irextractpolycoeff(\irexpression[2]')\\\\
    \irexpression[5] = \irextractpolyconst(\irexpression[1]')\qquad
    \irexpression[6] = \irextractpolyconst(\irexpression[2]')\\\\
    \irm_3 = \irm_1[\types \mapsto \float][\irshape \mapsto \irm_1(\irshape).append(\polys)][\irbroadcast \mapsto \irm_1(\irbroadcast).append(1)] \\\\ 
    \irm_4 = \irm_2[\types \mapsto \float][\irshape \mapsto \irm_2(\irshape).append(\polys)][\irbroadcast \mapsto \irm_2(\irbroadcast).append(1)] \\\\
    \irexpression[0]', \irexpression[3]', \irm_0 = \matchdims(\irexpression[0], \irexpression[3], \irm_0, \irm_3) \qquad
    \irexpression[0]^\dagger, \irexpression[5]^\dagger, \irm_0 = \matchdims(\irexpression[0], \irexpression[5], \irm_0, \irm_5) \\\\
    \irexpression[0]'', \irexpression[4]', \irm_3 = \matchdims(\irexpression[0]', \irexpression[4], \irm_0, \irm_4) \qquad
    \irexpression[0]^{\dagger\dagger}, \irexpression[6]^\dagger, \irm_5 = \matchdims(\irexpression[0]^\dagger, \irexpression[6], \irm_0, \irm_6) \\\\
    \irexpression[3]'', \irexpression[4]'', \irm_4 = \matchdims(\irexpression[3]', \irexpression[4]', \irm_0, \irm_3) \qquad
    \irexpression[5]^{\dagger\dagger}, \irexpression[6]^{\dagger\dagger}, \irm_6 = \matchdims(\irexpression[5]^\dagger, \irexpression[6]^\dagger, \irm_0, \irm_5) \\\\
    \irexpression[7] = \irternary(\irexpression[0]'', \irexpression[3]'', \irexpression[4]'') \qquad
    \irexpression[8] = \irternary(\irexpression[0]^{\dagger\dagger}, \irexpression[5]^{\dagger\dagger}, \irexpression[6]^{\dagger\dagger}) \\\\
    \irstatement = \irseq(\irseq(\irstatement[1], \irstatement[2]), \irstatement[3]) \qquad
    \irexpression = \ircombinesym(\irexpression[7], \irexpression[8]) \qquad 
    \irm = \irm_6
    }
    {
    \Gamma, \store_\irshape, \store_\irbroadcast, \fstore \models \expr_1 \ ? \ \expr_2 \ : \ \expr_3 \goesto \irstatement, \irexpression, \irm
    } 
    \\\\
    \inferrule*[lab = \textsc{Shape-ternary-symexp}]
    {
    \Gamma \vdash \expr_0 \ ? \ \expr_1 \ : \ \expr_2 : \symexp \\\\
    \Gamma, \store_\irshape, \store_\irbroadcast, \fstore \models \expr_0 \goesto \irstatement[0], \irexpression[0], \irm_0 \qquad
    \Gamma, \store_\irshape, \store_\irbroadcast, \fstore \models \expr_1 \goesto \irstatement[1], \irexpression[1], \irm_1 \qquad
    \Gamma, \store_\irshape, \store_\irbroadcast, \fstore \models \expr_2 \goesto \irstatement[2], \irexpression[2], \irm_2 \\\\
    \irm_1|_\types \in \{\float, \intt \} \implies \irexpression[1]' = \irconstsym(\irexpression[1]) \qquad
    \irm_1|_\types \in \{\typenoise \} \implies \irexpression[1]' = \irnoisesym(\irexpression[1]) \\\\
    \irm_2|_\types \in \{\float, \intt \} \implies \irexpression[2]' = \irconstsym(\irexpression[2]) \qquad
    \irm_2|_\types \in \{\typenoise \} \implies \irexpression[2]' = \irnoisesym(\irexpression[2]) \\\\
    \irexpression[3] = \irextractsymcoeff(\irexpression[1]')\qquad
    \irexpression[4] = \irextractsymcoeff(\irexpression[2]')\\\\
    \irexpression[5] = \irextractsymconst(\irexpression[1]')\qquad
    \irexpression[6] = \irextractsymconst(\irexpression[2]')\\\\
    \irm_3 = \irm_1[\types \mapsto \float][\irshape \mapsto \irm_1(\irshape).append(\syms)][\irbroadcast \mapsto \irm_1(\irbroadcast).append(1)] \\\\ 
    \irm_4 = \irm_2[\types \mapsto \float][\irshape \mapsto \irm_2(\irshape).append(\syms)][\irbroadcast \mapsto \irm_2(\irbroadcast).append(1)] \\\\
    \irexpression[0]', \irexpression[3]', \irm_0 = \matchdims(\irexpression[0], \irexpression[3], \irm_0, \irm_3) \qquad
    \irexpression[0]^\dagger, \irexpression[5]^\dagger, \irm_0 = \matchdims(\irexpression[0], \irexpression[5], \irm_0, \irm_5) \\\\
    \irexpression[0]'', \irexpression[4]', \irm_3 = \matchdims(\irexpression[0]', \irexpression[4], \irm_0, \irm_4) \qquad
    \irexpression[0]^{\dagger\dagger}, \irexpression[6]^\dagger, \irm_5 = \matchdims(\irexpression[0]^\dagger, \irexpression[6], \irm_0, \irm_6) \\\\
    \irexpression[3]'', \irexpression[4]'', \irm_4 = \matchdims(\irexpression[3]', \irexpression[4]', \irm_0, \irm_3) \qquad
    \irexpression[5]^{\dagger\dagger}, \irexpression[6]^{\dagger\dagger}, \irm_6 = \matchdims(\irexpression[5]^\dagger, \irexpression[6]^\dagger, \irm_0, \irm_5) \\\\
    \irexpression[7] = \irternary(\irexpression[0]'', \irexpression[3]'', \irexpression[4]'') \qquad
    \irexpression[8] = \irternary(\irexpression[0]^{\dagger\dagger}, \irexpression[5]^{\dagger\dagger}, \irexpression[6]^{\dagger\dagger}) \\\\
    \irstatement = \irseq(\irseq(\irstatement[1], \irstatement[2]), \irstatement[3]) \qquad
    \irexpression = \ircombinesym(\irexpression[7], \irexpression[8]) \qquad 
    \irm = \irm_6
    }
    {
    \Gamma, \store_\irshape, \store_\irbroadcast, \fstore \models \expr_1 \ ? \ \expr_2 \ : \ \expr_3 \goesto \irstatement, \irexpression, \irm
    } 
\end{array}
$
\caption{Shape analysis rules 3}
\label{fig:shapeanalysis3}
\end{figure}

\begin{figure}
\centering
$
\begin{array}{c}
    \inferrule*[lab = \textsc{Shape-map-symexp}]
    {
    \Gamma, \store_\irshape, \store_\irbroadcast, \fstore \models \expr \goesto \irstatement[1], \irexpression[1], \irm_1 \qquad 
    \Gamma \vdash \expr \sqsubseteq \symexp \\\\
    \irm_1|_\types = \typenoise \implies \irexpression[1]' = \irnoisesym(\irexpression[1]) \qquad
    \irm_1|_\types = \symexp \implies \irexpression[1]' = \irexpression[1] \\\\
    \forall i, j,  \irm'[i](\irshape)[j] = 1 \wedge  \irm'[i](\irbroadcast)[j] = \irm_1[i](\irshape)[j] \times \irm_1[i](\irbroadcast)[j] \\\\
    \irexpression[2] = \irmapnoise(\irexpression[1]) \qquad
    \irme[2] = \langle \typenoise, \false, [\syms], [1] \rangle \qquad
    \irm_2 = \irme[2] :: \irm' \\\\
    \irexpression[3] = \irmapcoeff(\irexpression[1]) \qquad
    \irme[3] = \langle \float, \false, [\syms], [1] \rangle \qquad
    \irm_3 = \irme[3] :: \irm_1 \\\\
    \irexpression[4] = \irextractsymconst(\irexpression[1]) \qquad 
    \irm_4 = \irm_1[\types \mapsto \float] \\\\
    \fstore(f) = (n, c), \expr' \qquad
    \sstore' = \sstore[n \mapsto \irexpression[2]][c \mapsto \irexpression[3]] \\\\ 
    \Gamma, \sstore', \store[\irshape], \store[\irbroadcast], \fstore \models \expr' \goesto \irstatement', \irexpression', \irm' \qquad 
    \irm' = \irme' :: \irme'' :: \irm'' \\\\
    \irexpression[5] = \irextractsymcoeff(\irexpression') \qquad 
    \irexpression[6] = \irextractsymconst(\irexpression') \\\\
    \irm_5 = \irme'[\types \mapsto \float][\irshape.append(\syms)][\irbroadcast.append(1)] :: \irme'' :: \irm'' \qquad 
    \irm_6 = \irme'[\types \mapsto \float] :: \irme'' :: \irm'' \\\\
    \irexpression[7] = \irreduce(\irexpression[5]) \qquad 
    \irexpression[8] = \irreduce(\irexpression[6]) \\\\
    \irm_7 = \irme'[\types \mapsto \symexp][\irshape.concat(\irme'(\irshape)[1:])][\irbroadcast.concat(\irme'(\irbroadcast)[1:]] :: \irm'' \qquad 
    \irm_8 = \irme''[\types \mapsto \float] :: \irm'' \\\\
    \irexpression[4]', \irexpression[8]', \irm_8' = \matchdims(\irexpression[4], \irexpression[8], \irm_4, \irm_8) \\\\
    \irexpression[9] = \irbinary(\irexpression[4], \irexpression[8]) \qquad 
    \irm_9 = \irm_8' \\\\
    \irstatement = \irseq(\irstatement[1], \irstatement') \qquad 
    \irexpression = \ircombinesym(\irexpression[7], \irexpression[8]') \qquad 
    \irm = \irm_9
    }
    {
    \Gamma, \store_\irshape, \store_\irbroadcast, \fstore \models \expr \cdot \map(f) \goesto \irstatement, \irexpression, \irm \\\\
    } 
\end{array}
$
\caption{Shape analysis rules 4}
\label{fig:shapeanalysis4}
\end{figure}
